# Supplementary material for: ReflectVLN: Training Vision-Language Navigation Agents with Reflective Reasoning
Source: arXiv:2607.12680 source file (2026-07-14)
Supplement: Supplementary file 1 [file 6_appendix.tex]

\section*{Supplementary Material}
\setcounter{section}{0}

This appendix provides additional comparisons and deployment notes. Training-data scale and on-demand vs.\ fixed intention triggering are reported in the main Experiments (Tables~\ref{tab:efficiency} and~\ref{tab:interval}).

\paragraph{Matched-regime snapshot.}
Table~\ref{tab:first_round} lists Val-Unseen scores for CorrectNav under its first flywheel round, together with DualVLN and ReflectVLN under their reported training settings (not the same flywheel protocol). Numbers align with CorrectNav$^{*}$ / DualVLN / Ours in Table~\ref{tab:r2r_rxr_valunseen}.

\begin{table}[t]
\centering
\small
\setlength{\tabcolsep}{6pt}
\begin{tabular}{l|ccc|ccc}
\toprule
& \multicolumn{3}{c|}{R2R-CE Val-Unseen} & \multicolumn{3}{c}{RxR-CE Val-Unseen} \\
& NE$\downarrow$ & SR$\uparrow$ & SPL$\uparrow$ & NE$\downarrow$ & SR$\uparrow$ & SPL$\uparrow$ \\
\midrule
CorrectNav (7B, 1st round) & 4.50 & 61.4 & 59.0 & 4.40 & 63.1 & 57.0 \\
DualVLN (7B) & \textbf{4.05} & \textbf{64.3} & 58.5 & 4.58 & 61.4 & 51.8 \\
Ours (3B) & 4.19 & 62.8 & \textbf{58.5} & \textbf{3.98} & \textbf{66.0} & \textbf{57.2} \\
\bottomrule
\end{tabular}
\caption{Supplementary score snapshot. CorrectNav uses the first flywheel round; DualVLN and Ours follow their reported settings.}
\label{tab:first_round}
\end{table}

\paragraph{Deployment variant (not used in main results).}
Replacing the execution-agent action head with a lightweight expert for edge deployment yields $\sim$17.50\,ms average step time on an NVIDIA Jetson Orin. This configuration differs from the main 3B VLM execution agent and is not used in the reported R2R/RxR tables.
